# Supplementary material for: Light-hole Exciton in Nanowire Quantum Dot
Source: arXiv:1612.01563 source file (2016-11-24)
Supplement: Supplementary file 1 [file Supplementary.pdf]

# Supplementary informations: Light-hole Exciton in Nanowire Quantum Dot

Mathieu Jeannin,[1,2] Alberto Artioli,[1,2] Pamela Rueda-Fonseca,[1,2,3] Edith Bellet-Amalric,[1,3] Kuntheak Kheng,[1,3] Régis André,[1,2] Serge Tatarenko,[1,2] Joël Cibert,[1,2] David Ferrand,[1,2] and Gilles Nogues[1,2]

[1]*Univ. Grenoble Alpes, F-38000 Grenoble, France*
[2]*CNRS, Inst. NEEL, "Nanophysique et semiconducteurs" group, F-38000 Grenoble, France*
[3]*CEA, INAC, "Nanophysique et semiconducteurs" group, F-38000 Grenoble, France*

## I. NANOWIRE AND QUANTUM DOT GROWTH

Nanowires are grown by molecular beam epitaxy in two interconnected ultra-high vacuum chambers over a 500 nm thick (111)B buffer layer of ZnTe[1,2]. Dewetted gold droplets are used as catalysts, and growth conditions are such that both longitudinal and lateral growth occur, leading to the final cone shape of the nanowire (tapering), with a core diameter ranging from 20 nm at the top to ≈200 nm at the base. Changing the temperature and atom fluxes allows then to grow a 20 nm thick ZnMgTe shell. The size of the QD and its Mn content are measured by energy dispersive spectroscopy on a nanowire from the same sample[3]. It confirms the Mn fraction of 10%. The QD has a diameter 8 nm and a length 12 nm.

(Cd,Mn)Te is a dilute magnetic semiconductor[4]: Cd atoms are randomly substituted by Mn atoms with a spin 5/2, giving rise to a magnetization in bulk semiconductors or to a magnetic moment $M$ in a quantum dot. At low temperature $T$ under an applied field $B$, $M$ follows a modified Brillouin function $M = M_{sat}B_{5/2}\left[\frac{5\mu_B B}{k_B(T+T_{AF})}\right]$, with $\mu_B$ the Bohr magneton, and where $M_{sat}$ and $T_{AF}$ are two phenomenological parameters which scale with the effective Mn concentration $x_{\text{eff}}$[4,5]: both $T_{AF}$ and $x_{\text{eff}}$ take into account the presence of antiferromagnetic interactions, and for instance with 10% Mn, $x_{\text{eff}} \simeq 4.0\%$, very close to its maximum value $x_{\text{eff}} \simeq 4.4\%$, and $T_{AF} \simeq 2.7$ K. The giant Zeeman splitting of electrons, LH and HH, with the magnetization oriented along the $z$-axis and saturated, are respectively given by $SN_0x_{\text{eff}}\alpha$, $SN_0x_{\text{eff}}\beta/3$ and $SN_0x_{\text{eff}}\beta$, respectively, where $N_0$ is the cation density in CdTe and $S = \frac{5}{2}$ the Mn spin. The exchange integrals for electron and holes in (Cd,Mn)Te are well documented[6], $N_0\alpha = 0.22$ eV and $N_0\beta = -0.88$ eV. With these values, we expect a giant Zeeman shift of the LH exciton, at saturation, $E_{sat}^{(LH)} = SN_0x_{\text{eff}}(\alpha-\beta/3)$ =25 meV (note that the dipole is along the $z$-axis, hence this line is not the line detected usually, i.e., in the $z$-direction with a small aperture), and $E_{sat}^{(HH)} = SN_0x_{\text{eff}}(\alpha-\beta)$ =55 meV for the HH exciton.

## II. EXPERIMENTAL SETUP

The cathodoluminescence system consists in a FEI Inspect F50 Schottky Field emission scanning electron microscope equipped with a Everhart-Thornley secondary electron detector and a custom cathodoluminescence system fitted with a GATAN cryogenic stage. The sample is mounted on a vertical sample holder to allow for cathodoluminescence at grazing incidence with respect to the sample surface.

Low temperature magneto-optical spectroscopy is carried out in a different cryostat than the Fourier microscopy one. Excitation conditions are similar. Microphotoluminescence spectra are recorded using a 46 cm Jobin-Yvon spectrometer coupled to a CCD camera. The as-grown sample mounted on piezo-scanners and the objective ($NA = 0.4$) are placed at cryogenic temperature ($T = 10$ K) in the middle of a 0-11 T solenoid magnet. The magnetic field is applied along the nanowire axis oriented parallel to the optical axis (Faraday configuration). We record simultaneously both circular polarisation of the emission lines using a $\lambda/4$ wave plate and a linear polarisation divider.

In the Fourier microscopy setup, a 2 μW continuous wave (CW) solid-state laser at 488 nm is used for excitation. The collection objective is a Zeiss EC Plan-Neofluar 40×, $NA = 0.75$, and the PL signal is detected by a CCD camera (Andor Newton 920). The objective is mounted on a piezo-scanning stage in front of the cryostat in a confocal microscopy setup.

The experimental setup for the Fourier plane microscopy experiment is sketched in Fig. 1. The excitation laser is a continuous wave laser emitting at 488 nm. A set of half wave plates and a polarising cube allow to excite the sample with a well defined polarisation state. A confocal microscopy scheme is employed, and the reflected laser signal is filtered by a long-pass filter. The collected fluorescence can be sent to a spectrometer or a CCD camera with a large active area for Fourier imaging using a flip mirror.

The Fourier imaging scheme is presented in figure 2. It consists in the addition of a lens in the usual confocal microscopy setup to image the back focal plane of the microscope objective. A linear polariser can be intrduced in the light path to perform the polarization-resolved measurements.

A photon emitted in the direction $(\theta, \varphi)$ is then converted by the microscope objective, and detected in the CCD camera plane. The electric field components are therefore transformed from spherical components

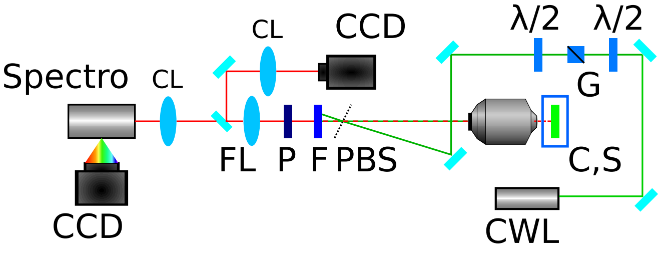


Figure 1. **Optical setup for microphotoluminescence and Fourier plane imaging experiments.**
$\lambda/2$: half-wavelength retardation plate, C: Cryostat, CL: Collection Lens, CWL: Continuous wave laser, F: Laser filter, FL: Fourier lens (movable), G: Glan-Thomson polarizing cube, P: Polarizer, PBS: pellicle beam-splitter (10% reflection), S: Sample. The objective is a Zeiss LD Plan-Neofluar 63x 0.75 NA objective. The Fourier lens is mounted on a removable translation stage for precise alignment. The mirror after the Fourier lens is flippable.

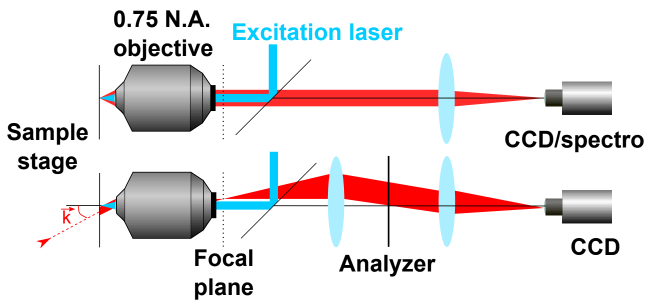


Figure 2. **Fourier plane imaging principle.**
In opposition with conventional confocal microscopy (top) in which one images directly the sample plane, Fourier imaging necessitates insertion of an additional lens with its object focal plane conjugated with the microscope objective image focal plane, transforming wavevectors into position in the detection plane (CCD) A linear polarizer (analyzer) can be inserted in the light path.

$(E_\theta, E_\varphi)$ into Cartesian components $(E_x, E_y)$ as follows:

$$E_x = E_\theta \cos\varphi - E_\varphi \sin\varphi$$
$$E_y = E_\theta \sin\varphi + E_\varphi \cos\varphi$$

A linear polariser can be inserted with an azimuthal angle $\varphi_p$ to perform polarization-resolved Fourier imaging, which then projects the transmitted linearly polarized electric field as shown into :

$$E_t = \begin{pmatrix} E\cos\left(\varphi - \varphi_p\right)\cos\varphi_p \\ E\cos\left(\varphi - \varphi_p\right)\sin\varphi_p \end{pmatrix} \tag{1}$$

The measurement of the objective's collection efficiency was performed by sending a small (50 µm in diameter), collimated laser beam with a defined angle through the microscope objective and measuring its intensity on the CCD camera. Repeating this operation for a large set of angles allows us to map the collection efficiency of

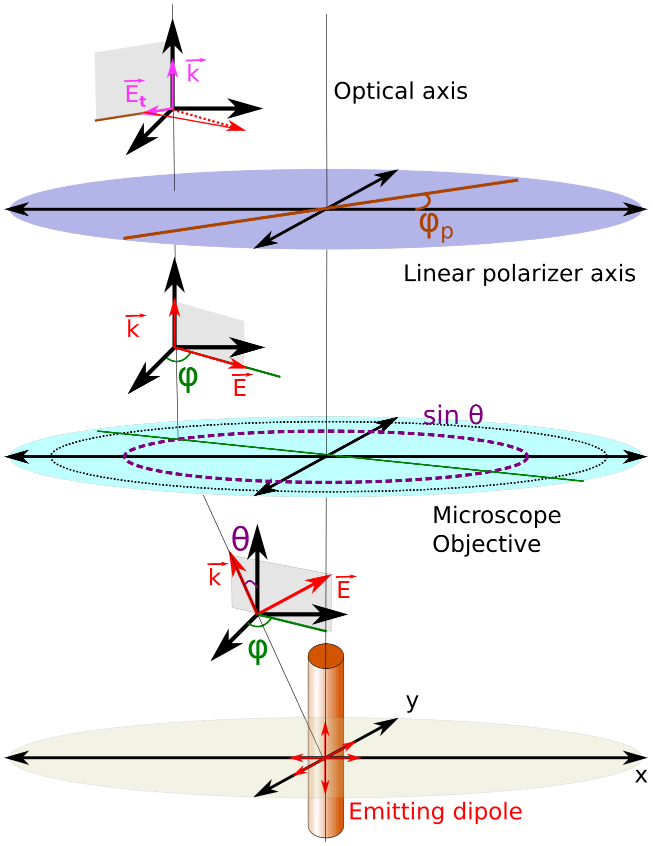


Figure 3. **Coordinated and conventions**.
Schematic of the coordinates conversion introduced in the Fourier plane.

the microscope objective as a function of collection angle $\theta$. It was further assumed that this collection efficiency was of rotational symmetry with respect to the optical axis.

## III. THEORETICAL FRAMEWORK

### Eigenstates and mixing

The eigenstates of $\mathcal{H}$ in the principal axes, [see Eq. (A3) of main article], are easily written by defining $\epsilon$ by $\tan(\epsilon) = \frac{2\rho_0}{\Delta_{LH0}}$. The mixed states $|\tilde{m}\rangle$ are formed upon only two pure states $|m\rangle$:

$$\left|\widetilde{+3/2}\right\rangle = \cos\frac{\epsilon}{2}\left|+3/2\right\rangle - \sin\frac{\epsilon}{2}\left|-1/2\right\rangle$$
$$\left|\widetilde{-1/2}\right\rangle = \cos\frac{\epsilon}{2}\left|-1/2\right\rangle + \sin\frac{\epsilon}{2}\left|+3/2\right\rangle \tag{2}$$

Note that the condition that $A_{z_0z_0}$ is the eigenvalue with the largest absolute value implies that $|\epsilon| < \pi/6$. At $\epsilon = \pi/6$, $A_{y_0y_0} = -A_{z_0z_0}$, $A_{x_0x_0} = 0$, and the eigenstates

are balanced (symmetrical and antisymmetrical) superpositions of light-holes and heavy-holes quantized along $x_0$. Beyond that value, $A_{y_0y_0}$ has the highest absolute value and the quantization axis must be taken along $y_0$.

With $\frac{\epsilon}{2} < \frac{\pi}{12}$, the first order of perturbation is generally sufficient. For instance, the light hole exciton ground state can be expressed in the laboratory frame as follows:

$$|X_{LH}\rangle \simeq |{+1/2}\rangle_h |{-1/2}\rangle_e + \beta\, |{-3/2}\rangle_h |{-1/2}\rangle_e + \gamma\, |{+3/2}\rangle_h |{-1/2}\rangle_e \quad (3)$$

with $|\gamma| = |\frac{\sigma}{\Delta E}|$ and $|\beta| = |\frac{\rho}{\Delta E'}|$, where $\Delta E$ (resp. $\Delta E'$) is the energy difference between $|+1/2>$ and $|+3/2>$ (resp. $|+1/2>$ and $|-3/2>$) hole levels. At zero field, $\Delta E = \Delta E' = \Delta_{LH}$; in the presence of a giant Zeeman effect, they can differ significantly.

### Emission diagram and polarization

In a direct-gap semiconductor such as GaAs or CdTe, the optical transitions result from the electric dipole between the electron state at the top of the valence band and the holes at the bottom of the conduction band. In term of electron-hole states, they can be summarized as follows[7]:

$$\begin{aligned}
\left\langle \frac{3}{2} \middle| \mathbf{p} \middle| S_- \right\rangle &= \frac{1}{\sqrt{2}}(\mathbf{p_x} + i\mathbf{p_y}) = \sigma^+ \\
\left\langle \frac{1}{2} \middle| \mathbf{p} \middle| S_- \right\rangle &= \sqrt{\frac{2}{3}}\mathbf{p_z} = \pi\sqrt{\frac{2}{3}} \\
\left\langle -\frac{1}{2} \middle| \mathbf{p} \middle| S_- \right\rangle &= -\frac{1}{\sqrt{6}}(\mathbf{p_x} - i\mathbf{p_y}) = \frac{-1}{\sqrt{3}}\sigma^- \\
\left\langle -\frac{3}{2} \middle| \mathbf{p} \middle| S_+ \right\rangle &= \frac{-1}{\sqrt{2}}(\mathbf{p_x} - i\mathbf{p_y}) = -\sigma^- \\
\left\langle -\frac{1}{2} \middle| \mathbf{p} \middle| S_+ \right\rangle &= \sqrt{\frac{2}{3}}\mathbf{p_z} = \pi\sqrt{\frac{2}{3}} \\
\left\langle \frac{1}{2} \middle| \mathbf{p} \middle| S_+ \right\rangle &= \frac{1}{\sqrt{6}}(\mathbf{p_x} + i\mathbf{p_y}) = \frac{1}{\sqrt{3}}\sigma^+ \quad (4)
\end{aligned}$$

In the absence of mixing, the selection rules in Fig. 1b of the main text follow.

In the presence of a magnetic field applied along the quantization axis (Fig. 4 in the main text), the circular polarization rate $S_3 = \frac{I_{\sigma^+} - I_{\sigma^-}}{I_{\sigma^+} + I_{\sigma^-}}$ expected for the light hole exciton line can be calculated using Eq. 3; it takes the form:

$$S_3 \simeq \frac{3f_{\sigma\pi}\gamma^2}{2 + 3f_{\sigma\pi}\gamma^2}$$

where $f_{\sigma\pi} \simeq 1.8$ is the ratio of collection efficiency of $\sigma$ and $\pi$ polarized light (see the main text) and integrated over the numerical aperture of the microscope objective (NA=0.4 in the present case). The large collection efficiency of $\sigma$ polarized light enhances the influence of the heavy hole components on the light hole exciton emission.

Finally, for an arbitrary mixing Hamiltonian $\mathcal{H}$, one can note that the emission diagram of a light hole exciton in vacuum remains a sum of three elementary orthogonal linear dipoles oriented along the principal axes ($x_0$, $y_0$, $z_0$), see Fig. 5 in main text. In a direction defined by the spherical angles $(\theta_0, \varphi_0)$ with respect to these axes, it takes the form:

$$I(\theta_0,\varphi_0) = d_{x_0}I_{x_0}(\theta_0,\varphi_0) + d_{y_0}I_{y_0}(\theta_0,\varphi_0) + d_{z_0}I_{z_0}(\theta_0,\varphi_0) \quad (5)$$

$I_{x_0}$, $I_{y_0}$ and $I_{z_0}$ are the intensity profiles of unitary linear dipoles given by:

$$\begin{aligned}
I_{x_0}(\theta_0,\varphi_0) &= 1 - \sin^2\theta_0\cos^2\varphi_0 \\
I_{y_0}(\theta_0,\varphi_0) &= 1 - \sin^2\theta_0\sin^2\varphi_0 \\
I_{z_0}(\theta_0,\varphi_0) &= \sin^2\theta_0.
\end{aligned}$$

$d_{x_0}$, $d_{y_0}$ and $d_{z_0}$ are proportional to the dipole magnitudes:

$$\begin{aligned}
d_{x_0} &= \left(\frac{1}{\sqrt{3}}\cos\frac{\epsilon}{2} - \sin\frac{\epsilon}{2}\right)^2 = \frac{4}{3}\cos^2(\frac{\epsilon}{2} + \frac{\pi}{3}) \\
d_{y_0} &= \left(\frac{1}{\sqrt{3}}\cos\frac{\epsilon}{2} + \sin\frac{\epsilon}{2}\right)^2 = \frac{4}{3}\cos^2(\frac{\epsilon}{2} - \frac{\pi}{3}) \\
d_{z_0} &= \frac{2}{3}\cos^2\frac{\epsilon}{2}
\end{aligned}$$

with $\epsilon$ defined for Eq. 2. For $\epsilon = 0$, $d_{x_0}$, $d_{y_0}$ and $d_{z_0}$ are proportional to the light hole exciton oscillator strengthes schematized in Fig. 1b of the main text.

## IV. NUMERICAL SIMULATIONS IMPLEMENTATION

For an emitter in a nanowire, the dipole magnitudes can be reduced by dielectric screening. The screening is stronger for transverse dipoles than for longitudinal ones. Guiding effects may also affect the intensity profiles of the elementary dipoles. This numerical simulation step thus includes dielectric screening from the NW and guiding effects in the high index NW structure.

Calculation of the farfield radiation pattern are carried out with a finite element method (FEM) software (Comsol Multiphysics v4.1). The full NW geometry is determined from the SEM image of the NW (Fig. 2b of main article). The conical shape with the correct taper angle and the presence of the index-matched substrate are taken into account. The emitter is modelled as a linearly polarized point electric dipole. Perfectly matched layer boundary conditions are used to truncate the simulation space, about one wavelength away from the emitter. The simulated electric and magnetic fields are propagated to the far-field through the readily implemented algorithm, from which we obtain the 3 complex field components in the upper half-space. We have checked that the farfield is transverse with only two components $(E_\theta, E_\varphi)$ in sperical

coordinates. The latter are transformed by the collection objective into an electric field in the $(x, y)$ plane as follows:

$$E_x = E_\theta \cos\varphi - E_\varphi \sin\varphi$$
$$E_y = E_\theta \sin\varphi + E_\varphi \cos\varphi$$

The resulting complex functions $E_{x,y}(\boldsymbol{u}, \theta, \varphi)$, where $\boldsymbol{u} = \boldsymbol{x}, \boldsymbol{y}, \boldsymbol{z}$ is the direction of the oscillating dipole, are calculated for a limited set of $(\theta, \varphi)$ determined by the finite element software. We develop those functions onto the basis of the spherical harmonics $Y_{lm}(\theta, \varphi)$ with $l$ ranging from 0 to 4. The relative error between the simulation result and its fit by spherical harmonics is below 3% over the whole objective's numerical aperture. The farfield created by the linear combination $\boldsymbol{d} = d_x\boldsymbol{x} + d_y\boldsymbol{y} + d_z\boldsymbol{z}$, resulting from the transition matrix elements (Eq. 4) between the electron state and the ground state of the valence band mixing Hamiltonian of Eq. (A1) in main article, is hence straightforwardly calculated in any direction $(\theta, \varphi)$ by using the proper linear combination of spherical harmonics.

In the case of the QD, we only consider the dipole at a fixed location corresponding to the QD position determined by cathodoluminescence (Fig. 2 of main text). In the case of the ZnTe core emission, we further incoherently sum the emission patterns for several emitter positions along the NW axis, weighted by the CL signal measured in Fig. 2 in the main text. The polarised emission diagrams and Stokes parameters diagrams are obtained by projecting the resulting electric field components $E_x$ and $E_y$ on the polariser directions and computing the correspondig intensity. The intensity maps are then corrected for the experimentally determined collection efficiency of the microscope objective (see the next paragraph).

The determination of the mixing parameters is separated in two steps, starting by the determination of the mixing amplitudes before finding the phase of each term. As noted in the main text, the effect of $\sigma/\Delta_{LH}$ can be measured by the power imbalance between the lobes in the polarization-resolved diagrams, and the one of $\rho/\Delta_{LH}$ by the magnitude of the Stokes parameters integrated over the whole numerical aperture. We thus fix the magnitudes of the mixing terms to match the experimental values. The phase term $\psi$ appears in the respective signs of $S_1$ and $S_2$ integrated over the whole numerical aperture. The phase term $\chi$ is responsible for the azimuthal direction of power imbalance in the unpolarised an polarisation-resolved diagrams. Using the previously determined amplitudes of the mixing terms, we compute the radiation patterns varying both phases to match the experimental values.

For comparison with the radiation patterns of the elementary dipoles in an homogeneous medium shown in Fig. 1 of the main text, we present in Fig. 4 the simulated radiation patterns with the determined mixing parameters but without the correction for the collection efficiency of the microscope objective. The high angular divergence of the $\pi$ transition is clearly visible in the simulated patterns for the light-hole emission. The lower angular divergence of the heavy-hole transition as compared with the expected pattern in an homogeneous medium arises from the guiding effect due to the high refractive index of the nanowire.

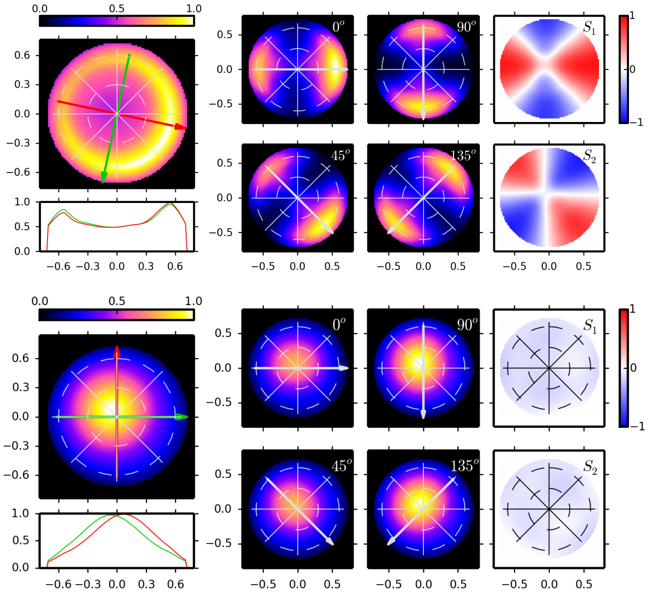


Figure 4. **Simulated radiation pattern without objective correction.**
Simulated radiation patterns using the same mixing parameters than the ones presented in the main text, without the collection efficiency correction from the microscope objective, for the QD emission (top) and the core emission (bottom). The emission from the QD is reinforced at very large angles and seems to diverge because of its $\pi$ character, while the one from the core remains well contained inside the numerical aperture due to its strong $\sigma^{\pm}$ character. Its low angular divergence can be attributed to the guiding effect form the NW structure.

[1] A. Artioli, A., P. Rueda-Fonseca, P., P. Stepanov, P., E. Bellet-Amalric, M. Den Hertog, C. Bougerol, Y. Genuist, F. Donatini, R. André, R., G. Nogues, and et al., Applied Physics Letters **103**, 222106 (2013).
[2] P. Rueda-Fonseca, E. Bellet-Amalric, R. Vigliaturo, M. den Hertog, Y. Genuist, R. André, R., E. Robin, A. Arti-

oli, P. Stepanov, D. Ferrand, and et al., Nano Lett. **14**, 1877–1883 (2014).

[3] P. Rueda-Fonseca, E. Robin, E. Bellet-Amalric, M. Lopez-Haro, M. Den Hertog, Y. Genuist, R. André, A. Artioli, S. Tatarenko, D. Ferrand, and et al., Nano Lett. **16**, 1637–1642 (2016).

[4] J. K. Furdyna, Journal of Applied Physics **64**, R29 (1988).

[5] J. A. Gaj, W. Grieshaber, C. Bodin-Deshayes, J. Cibert, G. Feuillet, Y. Merle d'Aubigné, and A. Wasiela, Physical Review B **50**, 5512–5527 (1994).

[6] J. Gaj, R. Planel, and G. Fishman, Solid State Communications **29**, 435–438 (1979).

[7] G. Fishman, *Semi-Conducteurs, les Bases de la Théorie k.p*, edited by L. E. de l'Ecole Polytechnique (Les Editions de l'Ecole Polytechnique, 2010).
